# Supplementary material for: Disentangling Label Distribution for Long-tailed Visual Recognition
Source: arXiv:2012.00321 source file (2021-03-20)
Supplement: Supplementary file 1 [file 6_Confidence_Calibration_supp.tex]

\begin{figure*}
\begin{center}
\includegraphics[width=\textwidth]{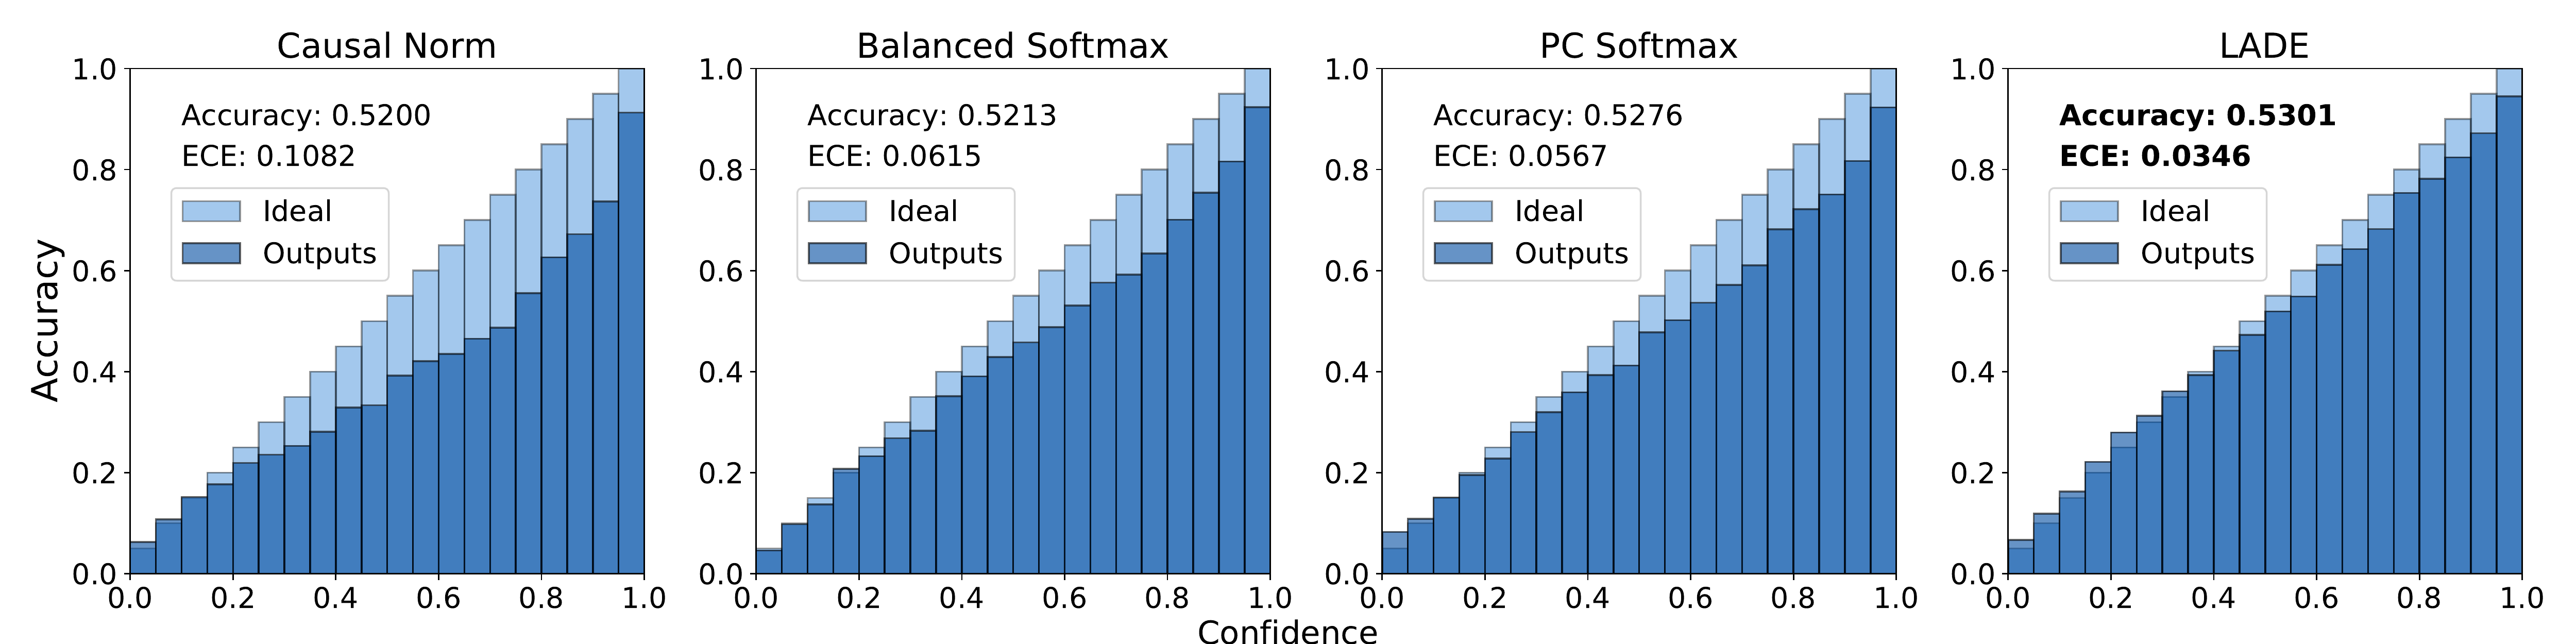}
\end{center}
\vspace{-10px}
\caption{Reliability diagrams of ResNeXt-50-32x4d~\cite{xie2017aggregated} on ImageNet-LT.
}
\label{fig:6_imagenet_confidence_calibration_fixed}
\end{figure*}
